# Supplementary material for: Oriented Active Solids
Source: arXiv:1812.01374 ancillary file (2018-12-04)
Supplement: Supplementary file 1 [file act_sol_supp.pdf]

# Active Solids: Supplementary

Ananyo Maitra[1,*] and Sriram Ramaswamy[2]
[1]LPTMS, CNRS, Univ. Paris-Sud, Université Paris-Saclay, 91405 Orsay, France
[2]Indian Institute of Science, 560012 Bangalore, India

## ACTIVE POLAR ELASTOMER ON A SUBSTRATE

In this section we present the detailed calculations for the dynamics of active polar elastomers on a substrate. As in the main paper, we start with the displacement field of the elastomer measured from an isotropic or unpolarised reference state $\bar{\mathbf{u}}(\mathbf{x}, t)$. We denote the polarisation field by $\mathbf{p}(\mathbf{x}, t)$ and the velocity field by $\mathbf{v}(\mathbf{x}, t)$. As mentioned in the main paper, since we consider permanently crosslinked systems, there is no motion of the structure without mass motion, i.e., no permeation. The density field $\rho$ is determined purely by the change in volume: $\delta\rho/\rho = -\nabla\cdot\bar{\mathbf{u}}$. Since, as we will demonstrate, the static structure factor of displacement fluctuations $\sim 1/q^2$ for all directions of the wavevector $\mathbf{q}$, at least within the linear theory, this immediately implies that the static structure factor of density fluctuations $\sim q^0$. That is, the density fluctuations scale as they would in an equilibrium system. This would be true even if we had considered a solid in which defect diffusion was allowed. That is, still there would have been no giant number fluctuation. The reason, as in other systems that simultaneously break rotation and translation symmetry, such as the smectic-A, is that the transverse fluctuations of the orientation field ($\mathbf{p}$ in our case) in the ordered phase are slaved to the fluctuations of the displacement field. This suppression of orientation fluctuations relative to the inhomogeneous background also leads to the suppression of number fluctuations. The only way systems breaking translation symmetry can have anomalous number fluctuations is if the orientational order is biaxial and orientation fluctuations about one of the axes is not slaved to displacement variables. This is possible for smectics, which have long-ranged positional correlations in only one direction: in a smectic-C there is orientational order both along the solid-like direction and in the plane transverse to it. The fluctuations about the transverse-plane orientational order are not suppressed by the smectic elasticity. Thus, an active smectic-C will display giant number fluctuations, with a region containing on average $N$ particles having a standard deviation scaling as $N^{(2+d)/2d} \sim N^{5/6}$ in dimension $d = 3$, where $N$ is the mean number. However, in systems that are solid-like in all directions, or all directions but one orientational fluctuations are always slaved to displacement fields even for biaxial systems, and number fluctuations are thus normal, of order $\sqrt{N}$.

As in the main paper, we define the linearised elastomer strain field $\mathsf{W} = \mathsf{C} + \Phi\mathsf{I}$, with components $W_{ij} = \partial_j\bar{u}_i + \partial_i\bar{u}_j$, with $\mathsf{C}$ and $\Phi$ being respectively the traceless and isotropic parts, and $\mathsf{I}$ the unit tensor. Since we will only concern ourselves with the linear theory the difference between left and right Cauchy-Green strain tensor is irrelevant for us [4]. We assume a simple relaxational dynamics for the polarisation field:

$$\partial_t\mathbf{p} = -\Gamma_p\frac{\delta F}{\delta\mathbf{p}}, \tag{1}$$

where $F$, to be defined below, is the free-energy functional governing relaxation to the equilibrium state in the absence of activity. In general, the dynamics of $\mathbf{p}$ also contains self-advective nonlinearities such as $\mathbf{p}\cdot\nabla\mathbf{p}$, advective nonlinearities such as $\mathbf{v}\cdot\nabla\mathbf{p}$ and couplings to the vorticity and the strain-rate. However, since we expect $\mathbf{p}$ to be slaved to the displacement variables, all such terms are irrelevant. Beyond this, the $\mathbf{p}$ can also respond directly to the velocity, and not its gradient in a system on a substrate, via a reversible coupling $\xi_p\mathbf{v}$ which has a counterpart $-\xi_p\delta F/\delta\mathbf{p}$ in the force balance equation. However, as we will work in the limit in which $\mathbf{v}$ has no independent dynamical evolution, but is simply determined in terms of the other fields in the problem through a constitutive law, its effect on $\mathbf{p}$ is only to shift the values of phenomenological constants. We will therefore ignore this "weathervane" term [1, 6, 7].

Since we consider permanently crosslinked elastomers with no permeation, the linear dynamics of the displacement field is simply

$$\dot{\bar{\mathbf{u}}} = \mathbf{v}, \tag{2}$$

In this section, we consider a solid on a high friction substrate and therefore obtain the force balance equation

$$\Gamma\mathbf{v} = \Gamma\upsilon\mathbf{p} + \Gamma\upsilon_1\mathbf{p}\cdot\mathsf{W} + \nabla\cdot\boldsymbol{\sigma}^a - \frac{\delta F}{\delta\mathbf{u}} \tag{3}$$

where $\Gamma\upsilon$ and $\Gamma\upsilon_1$ are the motility parameters, $\Gamma$ is the friction coefficient, and $\boldsymbol{\sigma}^a$ is an active stress

$$\sigma^a_{ij} = \zeta_1 D_{ij} + \zeta_2 p^2 \delta_{ij}, \tag{4}$$

where $D_{ij} = p_i p_j - (1/d)p^2\delta_{ij}$ with $d$ being the dimensionality. Other active stress terms proportional to $W_{ij}$ and $p_i p_k W_{jk}$ are allowed but doesn't lead to any qualitatively different physics and therefore we ignore them here. Further, all explicitly polar (i.e. odd under $\mathbf{p} \to -\mathbf{p}$) appear only at one higher order in gradients, and therefore, is subdominant to the stress terms we have retained. The free-energy

$$F = \int d^d\mathbf{x} \left[\frac{\lambda}{2}\left(\Phi - \frac{s}{\lambda}p^2\right)^2 + \mu\left(C_{ij} - \frac{t}{\mu}D_{ij}\right)\left(C_{ij} - \frac{t}{\mu}D_{ij}\right) + \frac{r}{2}p^2 + \frac{w}{4}p^4\right] \tag{5}$$

is symmetric under $\mathbf{p} \to -\mathbf{p}$ to lowest order in gradients, with explicitly polar terms appearing only at the next order. We now comment on the various couplings to velocity in the polarisation equation.

We now look for a homogeneously polarised state with a constant velocity. In principle, there are infinitely many states with this property and there is no universal criterion for state-selection out-of-equilibrium. In periodic systems, a vanishing dislocation speed would seem to be a reasonable criterion. However, an equivalent criteria in an amorphous system is difficult to formulate. We choose this state for two reasons: i. fluctuations about this state contain all terms allowed by the spatial symmetries of the system, and thus the fluctuation spectrum we discuss would not be qualitatively modified even if the actual steady state is different and ii. this is the equilibrium state in the absence of activity and we study the effect of adding activity perturbatively to this state. Here we choose the state with $\mathbf{p} = p_0\hat{x}$, with $p_0^2 = |r|/w$, $C^0_{ij} = t/\mu D^0_{ij}$, $\Phi^0 = (s/\lambda)p_0^2$ which has a steady velocity $\mathbf{v} = v_0\hat{x} = (\upsilon p_0 + \upsilon_1 p_0 W^0_{xx})\hat{x}$.

Expanding $\mathbf{p} = (p_0 + \delta p)(\cos\theta\hat{x} + \sin\theta\hat{y}) \approx (p_0 + \delta p)\hat{x} + p_0\theta\hat{y}$, $C_{ij} = C^0_{ij} + \delta C_{ij}$, and $\Phi = \Phi^0 + \delta\Phi$, we find from (1)

$$p_0\delta p = \frac{s\delta\Phi + 2t\delta C_{xx}}{\bar{r}} \tag{6}$$

where $\bar{r} = w + (2s^2/\lambda) + 2(t^2/\mu)$ and

$$\theta = \frac{\mu}{tp_0^2}\delta C_{xy}. \tag{7}$$

As expected, the transverse fluctuations of the broken symmetry polarisation field are not soft and are instead slaved to $C_{xy}$.

Since we examine the fluctuations about this state, it is advantageous to transform to displacement and strain variables measured relative to this state instead of using $\bar{\mathbf{u}}$ and $\mathbf{C}$ and $\Phi$ which are defined relative to the isotropic state. The steady-state deformation tensor of the anisotropic state is $\mathbf{\Lambda}_0\mathbf{\Lambda}_0^T = 2\mathbf{W}^0 + \mathbf{I}$ where $\mathbf{\Lambda}_0$ is the deformation matrix of the homogeneously polarised state which we write as

$$\mathbf{\Lambda}_0\mathbf{\Lambda}_0^T = \begin{pmatrix} \Lambda_\parallel^2 & 0 \\ 0 & \Lambda_\perp^2 \end{pmatrix} \tag{8}$$

with $\Lambda_\parallel^2 = p_0^2(s/\lambda + t/\mu) + 1$ and $\Lambda_\perp^2 = p_0^2(s/\lambda - t/\mu) + 1$. The anisotropy is $\Lambda_\parallel^2 - \Lambda_\perp^2 = (2t/\mu)p_0^2$. We also define $\mathcal{R} = \Lambda_\parallel^2/\Lambda_\perp^2$. The deviations about the polarised state are characterised by the strain tensor $\delta\mathbf{W} = (1/2)(\mathbf{\Lambda}\mathbf{\Lambda}^T - \mathbf{\Lambda}_0\mathbf{\Lambda}_0^T)$ where $\mathbf{\Lambda}$ is the deformation matrix for the fluctuating state. We define the displacement field $\mathbf{u}$ and the strain tensor $\boldsymbol{\eta}$ about the homogeneously polarised reference state. Defining the projection operators $\mathbf{P}_\parallel = \hat{p}\hat{p}$ and $\mathbf{P}_\perp = \mathbf{I} - \hat{p}\hat{p}$, where $\hat{p} = (\cos\theta\hat{x} + \sin\theta\hat{y})$ is the unit vector along $\mathbf{p}$, we can decompose the strain tensor as $\mathbf{P}_\parallel \cdot \boldsymbol{\eta} \cdot \mathbf{P}_\parallel = \eta_{\parallel\parallel}\hat{p}\hat{p}$ where, to lowest order, $\eta_{\parallel\parallel} \approx \partial_x u_x = \eta_{xx}$, $\mathbf{P}_\parallel \cdot \boldsymbol{\eta} \cdot \mathbf{P}_\perp = \eta_{\parallel\perp}\hat{p}\hat{p}_\perp$ with $\hat{p}_\perp = (-\sin\theta\hat{x} + \cos\theta\hat{y})$ being a unit vector perpendicular to $\hat{p}$ and $\eta_{\parallel\perp} \approx (1/2)(\partial_x u_y + \partial_y u_x) = \eta_{xy}$, and $\mathbf{P}_\perp \cdot \boldsymbol{\eta} \cdot \mathbf{P}_\perp = \eta_{\perp\perp}\hat{p}_\perp\hat{p}_\perp$ with $\eta_{\perp\perp} \approx \partial_y u_y = \eta_{yy}$. We further define the rotation angle $\Omega = (\partial_x u_y - \partial_y u_x)/2$. $\delta\mathbf{W}$ is related to $\nabla\mathbf{u}$ as $\delta W_{xx} = \Lambda_\parallel^2\eta_{xx}$, $\delta W_{xy} = (1/2)(\Lambda_\perp^2\partial_y u_x + \Lambda_\parallel^2\partial_x u_y)$ and $\delta\Phi = \Lambda_\parallel^2\partial_x u_x + \Lambda_\perp^2\partial_y u_y$. Using the definitions of $\boldsymbol{\eta}$ and $\Omega$, $\theta$ can be rexpressed as

$$\theta = \Omega + \beta^{-1}\eta_{xy} \tag{9}$$

where $\beta = (\mathcal{R} - 1)/(\mathcal{R} + 1)$, while

$$p_0\delta p = \frac{1}{\bar{r}}[(t+s)\Lambda_\parallel^2\eta_{xx} + (t-s)\Lambda_\perp^2\eta_{yy}] \tag{10}$$

Eliminating the massive $\delta p$ fluctuations, we can rewrite the free energy in terms of $\theta$ and $\boldsymbol{\eta}$ as

$$F = \frac{1}{2}\int d^2\mathbf{x} B_1\eta_{xx}^2 + B_2\eta_{yy}^2 + B_3\eta_{xx}\eta_{yy} + B_4[\eta_{xy} - \beta(\theta-\Omega)]^2 \tag{11}$$

where

$$B_1 = \frac{\Lambda_\parallel^4}{\bar{r}}\left[\frac{2t^2\lambda}{\mu} - 4st + \frac{2s^2\mu}{\lambda} + w(\lambda+\mu)\right] \tag{12}$$

$$B_2 = \frac{\Lambda_\perp^4}{\bar{r}}\left[\frac{2t^2\lambda}{\mu} + 4st + \frac{2s^2\mu}{\lambda} + w(\lambda+\mu)\right] \tag{13}$$

$$B_3 = \frac{2\Lambda_\perp^2\Lambda_\parallel^2}{\bar{r}}\left[\frac{2t^2\lambda}{\mu} - \frac{2s^2\mu}{\lambda} + w(\lambda-\mu)\right] \tag{14}$$

$$B_4 = \mu(\mathcal{R}+1)\Lambda_\perp^4. \tag{15}$$

The form of this free energy immediately demonstrates that there is no energy cost for shear deformations to harmonic order in equilibrium polar elastomers. This implies that such elastomers can not support a static shear, which is a hallmark property of solids.

We now project the force balance equation (3) parallel and transverse to the polarisation direction. First, the components of the propulsive force $\mathbf{f}_p = \Gamma(\upsilon\mathbf{p} + \upsilon_1\mathbf{p}\cdot\mathbf{W})$ are

$$\hat{p}\cdot\mathbf{f}_p = f_{p\parallel} = \cos\theta f_{px} + \sin\theta f_{py} \overset{\text{lin}}{=} \Gamma(\upsilon p_0 + \upsilon_1 p_0 W_{xx}^0)\hat{x} + \Gamma(\upsilon\delta p + \upsilon_1\delta p W_{xx}^0 + \upsilon_1 p_0\delta W_{xx})\hat{x} = \Gamma v_0 + a_1\partial_x u_x + a_2\partial_y u_y \tag{16}$$

where

$$a_1 = p_0\upsilon_1\Lambda_\parallel^2 + \frac{(s+t)\Lambda_\parallel^2}{2p_0\bar{r}}[2\upsilon + \upsilon_1(\Lambda_\parallel^2 - 1)] \tag{17}$$

and

$$a_2 = \frac{(t-s)\Lambda_\parallel^2}{2p_0\bar{r}}[2\upsilon + \upsilon_1(\Lambda_\parallel^2 - 1)], \tag{18}$$

$$\begin{aligned}\hat{p}_\perp\cdot\mathbf{f}_p = f_{p\perp} &= -\sin\theta f_{px} + \cos\theta f_{py} \overset{\text{lin}}{=} -\theta\Gamma(\upsilon p_0 + \upsilon_1 p_0 W_{xx}^0) + f_{ay} \\ &= \Gamma[\upsilon p_0\theta + \upsilon_1\delta W_{xy}p_0 + W_{yy}^0 p_0\theta - \theta\upsilon p_0 - \theta\upsilon_1 W_{xx}^0 p_0] = \Gamma\upsilon_1 p_0(\delta W_{xy} - 2\theta C_{xx}^0).\end{aligned} \tag{19}$$

Now, $C_{xx}^0 = (t/2\mu)p_0^2$ and $\theta = (\mu/tp_0^2)\delta C_{xy} = (\mu/tp_0^2)\delta W_{xy}$. Therefore, $2\theta C_{xx}^0 = \delta W_{xy}$ and $f_{a\perp} = 0$. This implies that there is no propulsive force in the direction transverse to the polarisation in a spontaneously symmetry broken polar elastomer. This is in distinction to externally driven solids [3]. This is another manifestation of the Anderson-Higgs mechanism that eliminates the energy cost for shear deformations. Since the strain asymmetry is produced by a spontaneously symmetry-broken $\mathbf{p}$, the any deviation of $\mathbf{W}$ away from $\mathbf{pp}$ relaxes in a short timescale – the symmetry is not under *independent* rotations of the solid and $\mathbf{p}$ but under *joint* rotations. Therefore, $\mathbf{W}\cdot\mathbf{p}$ is purely along $\mathbf{p}$ and has no component transverse to it. A similar argument for driven polar smectics should imply that there is no force $\propto \nabla_\perp u$, where $u$ is the displacement field of the smectic, in the direction transverse to the layers. Such a force would have implied that a uniform tilt of the smectic layers would drive a current transverse to the layers and which essentially would have implied the presence of an external symmetry breaking field such as a gravitational field.

Next, we decompose the active force originating from the stress:

$$\mathbf{f}_\sigma \overset{\text{lin}}{=} p_0\nabla\cdot\begin{pmatrix}(\zeta_1+2\zeta_2)\delta p & \zeta_1 p_0\theta \\ \zeta_1 p_0\theta & -(\zeta_1-2\zeta_2)\delta p\end{pmatrix} \tag{20}$$

This implies

$$\hat{p}\cdot\mathbf{f}_\sigma = f_{\sigma\|} \overset{\text{lin}}{=} \frac{(\zeta_1+2\zeta_2)}{\bar{r}}\partial_x[(t+s)\Lambda_\|^2\eta_{xx} + (t-s)\Lambda_\perp^2\eta_{yy}] + \zeta_1 p_0^2(\partial_y\Omega + \beta^{-1}\partial_y\eta_{xy}) \tag{21}$$

$$\hat{p}_\perp\cdot\mathbf{f}_\sigma = f_{\sigma\perp} \overset{\text{lin}}{=} -\frac{(\zeta_1-2\zeta_2)}{\bar{r}}\partial_y[(t+s)\Lambda_\|^2\eta_{xx} + (t-s)\Lambda_\perp^2\eta_{yy}] + \zeta_1 p_0^2(\partial_x\Omega + \beta^{-1}\partial_x\eta_{xy}) \tag{22}$$

Finally, the elastic force $f_{el} = -\delta F/\delta\mathbf{u}$ can be decomposed to yield

$$f_{el\|} = B_1\partial_x\eta_{xx} + \frac{B_3}{2}\partial_x\eta_{yy} \tag{23}$$

$$f_{el\perp} = B_3\partial_y\eta_{yy} + \frac{B_3}{2}\partial_y\eta_{xx} \tag{24}$$

Note that the active force (21) and (22) lead to a resistance to shear deformations if $\zeta_1\beta^{-1} > 0$ i.e. if $(\zeta_1/t)\mu(1+s/\lambda) > 0$. This implies that when $\zeta_1 > 0$ ($\zeta_1 < 0$), i.e. the filaments generate contractile (extensile) stresses, the solid can support a static shear if $t > 0$ ($t < 0$) i.e., the filaments align parallel (perpendicular) to the elastic mesh. However, when $\zeta_1 > 0$ ($\zeta_1 < 0$), the oreintationally ordered solid is destabilised if $t < 0$ ($t > 0$) i.e., the filaments align perpendicular (parallel) to the elastic mesh.

We now transform to a frame moving with the mean velocity of the solid $v_0\hat{x}$ and project $\partial_t\mathbf{u}$ parallel and perpendicular to the polarisation direction.

$$\hat{p}\cdot\mathbf{v} = \cos\theta v_x + \sin\theta v_y \approx \partial_t u_x + \theta\partial_t u_y \overset{\text{lin}}{=} \partial_t u_x \tag{25}$$

$$\hat{p}_\perp\cdot\mathbf{v} = -\sin\theta v_x + \cos\theta v_y \approx -\theta\partial_t u_x + \partial_t u_y \overset{\text{lin}}{=} \partial_t u_y \tag{26}$$

where the last relation in (26) holds since in the frame moving with the mean speed of the solid, $\theta\partial_t u_x$ has no linear part. With all of this, we can now write down the equations for $\mathbf{u}$ fluctuations in the co-moving frame of the solid:

$$\partial_t u_x = a_1\partial_x u_x + a_2\partial_y u_y + b_1\partial_x^2 u_x + b_2\partial_y^2 u_x + b_3\partial_x\partial_y u_y \tag{27}$$

$$\partial_t u_y = b_4\partial_x^2 u_y + b_5\partial_y^2 u_y + b_6\partial_x\partial_y u_x \tag{28}$$

where the $b_i$ are

$$b_1 = \frac{1}{\Gamma}\left[B_1 + \frac{(t+s)\Lambda_\|^2}{\bar{r}}(2\zeta_2+\zeta_1)\right] \tag{29}$$

$$b_2 = \frac{p_0^2\zeta_1}{2\Gamma}(\beta^{-1}-1) \tag{30}$$

$$b_3 = \frac{1}{2\Gamma}\left[B_3 + p_0^2\zeta_1(\beta^{-1}+1) + \frac{2(t-s)\Lambda_\perp^2}{\bar{r}}(2\zeta_2+\zeta_1)\right] \tag{31}$$

$$b_4 = \frac{p_0^2\zeta_1}{2\Gamma}(\beta^{-1}+1) \tag{32}$$

$$b_5 = \frac{1}{\Gamma}\left[B_2 + \frac{(t-s)\Lambda_\perp^2}{\bar{r}}(2\zeta_2-\zeta_1)\right] \tag{33}$$

$$b_6 = \frac{1}{2\Gamma}\left[B_3 + p_0^2\zeta_1(\beta^{-1}-1) + \frac{2(t+s)\Lambda_\|^2}{\bar{r}}(2\zeta_2-\zeta_1)\right] \tag{34}$$

This yields the eigenfrequencies

$$\omega_\pm = \begin{cases} q_x \ll q_y^2 \begin{cases} -b_2 q_y^2 + i\left(a_1 + \frac{a_2 b_6}{|b2-b5|}\right) q_x \\ -b_5 q_y^2 - i\frac{a_2 b_6}{|b2-b5|} q_x \end{cases} \\ q_x \gtrsim q_y^2 \begin{cases} i a_1 q_x - b_1 q_x^2 - b_2 q_y^2 - \frac{a_2}{a_1} b_6 q_y^2 \\ -b_4 q_x^2 - b_5 q_y^2 + \frac{a_2}{a_1} b_6 q_y^2 \end{cases} \end{cases} \tag{35}$$

Since both $b_2$ and $b_4$ are purely controlled by the active coefficient $\zeta_1$, the system is unstable when $\zeta_1 < 0$ and $\beta^{-1} > 1$ or when $\zeta_1 > 0$ and $\beta^{-1} < -1$. This instability is present in apolar elastomers as well. However, motility does introduce the possibility of a further instability when the magnitude of $\zeta_1$ is small: if the motility coefficients $a_2$ and $a_1$ have opposite signs then for small enough value of $b_2$, the system is destabilised.

We now explicitly show that when the solid is stable, the static structure factor of $\mathbf{u}$ fluctuations always scale as $1/q^2$ in all directions. For $q_x \ll q_y^2$, the static structure factors are simply

$$\langle u_x(q,t) u_x(-q,t)\rangle = \frac{T}{b_2 q_y^2}; \quad \langle u_y(q,t) u_y(-q,t)\rangle = \frac{T}{b_5 q_y^2} \tag{36}$$

while for $q_x \gtrsim q_y^2$, they are

$$\langle u_x(q,t) u_x(-q,t)\rangle = \frac{T}{b_1 q_x^2 + [b_2 + (a_2/a_1) b_6] q_y^2}; \quad \langle u_y(q,t) u_y(-q,t)\rangle = \frac{T}{b_4 q_x^2 + [b_5 - (a_2/a_1) b_6] q_y^2} \tag{37}$$

This demonstrates that the static structure factors scale as $1/q^2$ in all directions for $q \to 0$.

## ACTIVE APOLAR ELASTOMER ON A SUBSTRATE

We assume a simple relaxational dynamics for the apolar order parameter

$$\partial_t \mathbf{Q} = -\Gamma_Q \frac{\delta F}{\delta \mathbf{Q}}. \tag{38}$$

The possible velocity couplings that could appear in this equation are all irrelevant. In particular, even in systems on substrates, there is no linear coupling to the velocity as opposed the velocity gradient, in contrast to the polar fluids (the equivalent term is non-linear in this case $\propto \mathbf{v}\mathbf{v} - (1/2)v^2$ which has no linear part even in the ordered phase since by symmetry, apolar systems do not self-propel). The displacement dynamics reads

$$\dot{\mathbf{u}} = \mathbf{v}, \tag{39}$$

$$\Gamma \mathbf{v} = \tilde{\zeta}_1 \nabla \cdot \mathbf{Q} + \tilde{\zeta}_2 \mathbf{Q} \cdot (\nabla \cdot \mathbf{Q}) - \frac{\delta F}{\delta \bar{\mathbf{u}}} \tag{40}$$

We also ignore an active component to the isotropic stress propotional to $Q_{ij} Q_{ij}$. The Free energy for an apolar elastomer is

$$F = \int d^2\mathbf{x} \left[\frac{\lambda}{2}\left(\Phi - \frac{s}{\lambda} Q_{ij} Q_{ij}\right)^2 + \mu\left(C_{ij} - \frac{t}{\mu} Q_{ij}\right)\left(C_{ij} - \frac{t}{\mu} Q_{ij}\right) + \frac{r}{2} Q_{ij} Q_{ij} + \frac{w}{4}(Q_{ij} Q_{ij})^2\right] \tag{41}$$

We consider a steady state with

$$\mathbf{Q}^0 = \frac{S_0}{2}\begin{pmatrix} 1 & 0 \\ 0 & -1 \end{pmatrix} \tag{42}$$

$S_0^2 = 2r/w$, $\Phi^0 = (s/2\lambda) S_0^2$ and $C_{ij} = (t/\mu) Q_{ij}^0$. We now consider fluctuations about this steady state:

$$Q_{ij} = Q_{ij}^0 + \delta Q_{ij} = \frac{S_0 + \delta S}{2}\begin{pmatrix} 1 & 2\theta \\ 2\theta & -1 \end{pmatrix} \tag{43}$$

$$\delta S = \frac{2t}{\bar{w}}\delta C_{xx} + \frac{sS_0}{\bar{w}}\delta\Phi \tag{44}$$

and

$$\theta = \frac{\mu}{S_0 t}\delta C_{xy} \tag{45}$$

where $\bar{w} = S_0 s^2/\lambda + t^2/\mu + r$. As earlier, we now transform to a strain field defined about the anisotropic state whose parameters are $\Lambda_\parallel^2 = \frac{tS_0}{\mu} + \frac{s}{2\lambda}S_0^2 + 1$, $\Lambda_\perp^2 = -\frac{tS_0}{\mu} + \frac{s}{2\lambda}S_0^2 + 1$. This implies that $\Lambda_\parallel^2 - \Lambda_\perp^2 = \frac{2t}{\mu}S_0$. Again integrating out the $\delta S$ fluctuations, we obtain the free-energy in terms of the strain variables about the the anisotropic state $\boldsymbol{\eta}$ and the angle field $\Omega$:

$$F = \frac{1}{2}\int d^2\mathbf{x} B_1\eta_{xx}^2 + B_2\eta_{yy}^2 + B_3\eta_{xx}\eta_{yy} + B_4[\eta_{xy} - \beta(\theta - \Omega)]^2 \tag{46}$$

where

$$B_1 = \frac{\Lambda_\parallel^4}{\bar{w}}\left[\frac{t^2\lambda}{\mu} + S_0 s\left(\frac{s\mu}{\lambda} - 2t\right) + r(\lambda + \mu)\right] \tag{47}$$

$$B_2 = \frac{\Lambda_\perp^4}{\bar{w}}\left[\frac{t^2\lambda}{\mu} + S_0 s\left(\frac{s\mu}{\lambda} + 2t\right) + r(\lambda + \mu)\right] \tag{48}$$

$$B_3 = \frac{2\Lambda_\perp^2\Lambda_\parallel^2}{\bar{w}}\left[\frac{t^2\lambda}{\mu} - \frac{S_0 s^2\mu}{\lambda} + r(\lambda - \mu)\right] \tag{49}$$

$$B_4 = \mu(\mathcal{R} + 1)\Lambda_\perp^4. \tag{50}$$

$\delta S$ in terms of $\boldsymbol{\eta}$ is

$$\delta S = \frac{1}{\bar{w}}[(t + sS_0)\Lambda_\parallel^2\eta_{xx} + (t - sS_0)\Lambda_\perp^2\eta_{yy}] \tag{51}$$

and the angle director field is slaved to strain and rotation as

$$\theta = \Omega + \beta^{-1}\eta_{xy} \tag{52}$$

Now, as in the polar elastomer, we decompose the velocity field parallel and perpendicular to the ordering direction. The active force

$$\mathbf{f}_a \overset{\text{lin}}{=} \bar{\zeta}_1\nabla\cdot\begin{pmatrix}\delta S/2 & S_0\theta\\ S_0\theta & -\delta S/2\end{pmatrix} + \bar{\zeta}_2\frac{S_0}{2}\begin{pmatrix}1 & 0\\ 0 & -1\end{pmatrix}\cdot\nabla\cdot\begin{pmatrix}\delta S/2 & S_0\theta\\ S_0\theta & -\delta S/2\end{pmatrix} \tag{53}$$

This yields

$$f_{a\parallel} \overset{\text{lin}}{=} \left(\zeta_1 + \frac{\zeta_2 S_0}{2}\right)\left(\frac{1}{2}\partial_x\delta S + S_0\partial_y\theta\right) = \left(\zeta_1 + \frac{\zeta_2 S_0}{2}\right)\left[\partial_x\left\{\frac{(t + sS_0)\Lambda_\parallel^2}{2\bar{w}}\eta_{xx} + \frac{(t - sS_0)\Lambda_\perp^2}{2\bar{w}}\eta_{yy}\right\} + S_0\partial_y(\Omega + \beta^{-1}\eta_{xy})\right] \tag{54}$$

$$f_{a\perp} \overset{\text{lin}}{=} \left(\zeta_1 - \frac{\zeta_2 S_0}{2}\right)\left(S_0\partial_x\theta - \frac{1}{2}\partial_y\delta S\right) = \left(\zeta_1 - \frac{\zeta_2 S_0}{2}\right)\left[-\partial_y\left\{\frac{(t + sS_0)\Lambda_\parallel^2}{2\bar{w}}\eta_{xx} + \frac{(t - sS_0)\Lambda_\perp^2}{2\bar{w}}\eta_{yy}\right\} + S_0\partial_x(\Omega + \beta^{-1}\eta_{xy})\right]. \tag{55}$$

The elastic forces are

$$f_{el\parallel} = B_1\partial_x\eta_{xx} + \frac{B_3}{2}\partial_x\eta_{yy} \tag{56}$$

$$f_{el\perp} = B_3\partial_y\eta_{yy} + \frac{B_3}{2}\partial_y\eta_{xx} \tag{57}$$

Rescaling time by $\Gamma$, we therefore obtain the equations of motion

$$\partial_t u_x = \nu_1\partial_x^2 u_x + \nu_2\partial_y^2 u_x + \nu_3\partial_x\partial_y u_y \tag{58}$$

$$\partial_t u_y = \nu_4\partial_x^2 u_y + \nu_5\partial_y^2 u_y + \nu_6\partial_x\partial_y u_x \tag{59}$$

where the $b_i$ are

$$\nu_1 = \left[B_1 + \frac{(t+sS_0)\Lambda_{\parallel}^2}{4\bar{r}}(2\tilde{\zeta}_1 + \tilde{\zeta}_2 S_0)\right] \tag{60}$$

$$\nu_2 = S_0\frac{2\tilde{\zeta}_1 + \tilde{\zeta}_2 S_0}{4}(\beta^{-1} - 1) \tag{61}$$

$$\nu_3 = \frac{1}{2}\left[B_3 + \frac{(2\tilde{\zeta}_1 + \tilde{\zeta}_2 S_0)}{2}\left\{S_0(\beta^{-1}+1) + \frac{(t-sS_0)\Lambda_{\perp}^2}{2\bar{w}}\right\}\right] \tag{62}$$

$$\nu_4 = S_0\frac{2\tilde{\zeta}_1 - \tilde{\zeta}_2 S_0}{4}(\beta^{-1} + 1) \tag{63}$$

$$\nu_5 = \left[B_2 + \frac{(t-sS_0)\Lambda_{\perp}^2}{4\bar{w}}(-2\tilde{\zeta}_1 + \tilde{\zeta}_2 S_0)\right] \tag{64}$$

$$\nu_6 = \frac{1}{2}\left[B_3 + \frac{(2\tilde{\zeta}_1 - \tilde{\zeta}_2 S_0)}{2}\left\{S_0(\beta^{-1}-1) - \frac{(t+sS_0)\Lambda_{\parallel}^2}{2\bar{w}}\right\}\right] \tag{65}$$

Note that these equations are not only different from passive nematic elastomers, but are also distinct from passive uniaxial solids. Passive uniaxial solids would have had four independent coefficients which would have implied that $\nu_2 = \nu_4$ and $\nu_3 = \nu_6$. The general eigenfrequency that this yields is fairly complicated:

$$\omega_{\pm} = -\frac{iq^2}{2}\left[\{(\nu_1+\nu_4)\cos^2\phi + (\nu_2+\nu_5)\sin^2\phi\} \mp \sqrt{\{(\nu_1-\nu_4)\cos^2\phi + (\nu_2-\nu_5)\sin^2\phi\}^2 + 4\nu_3\nu_6\sin^2\phi\cos^2\phi}\right] \tag{66}$$

where $\phi$ is the angle that the wavevector makes with the ordering direction. However, the most interesting effect of activity can be studied by just focussing on the directions $q_x = 0$ and $q_y = 0$ i.e. transverse to and along the direction of ordering respectively, since these are the directions that are the softest in a passive apolar elastomer. In these directions, the $u_x$ and $u_y$ equations obviously decouple and the eigenvalues when $\phi = 0$ are $\{-\nu_1 q_x^2, -\nu_4 q_x^2\}$ while for $\phi = \pi/2$ are $\{-\nu_2 q_y^2, -\nu_5 q_y^2\}$. Now, due to the softness of nematic elastomers, both $\nu_2$ and $\nu_4$ are purely active. Both of them need to be positive to ensure stability. Noting that $\beta^{-1} > 1$ for positively uniaxial systems (i.e. for which $\Lambda_{\parallel}^2 > \Lambda_{\perp}^2$), we find that stability requires $\tilde{\zeta}_1 > |(\tilde{\zeta}_2 S_0/2)|$. If on the other hand $\Lambda_{\parallel}^2 < \Lambda_{\perp}^2$ i.e. the system is *negatively* uniaxial, which happens most naturally when $t$, the coefficient of the free-energy coupling between the deviatoric strain $\mathbf{C}$ and the apolar order parameter, $\mathbf{Q}$, stability requires that $\tilde{\zeta}_1 < -|(\tilde{\zeta}_2 S_0/2)|$. A negative $\tilde{\zeta}_1$ which denotes extensile stresses in this convention, destabilises a positively uniaxial system (i.e., systems in which the nematogens align along the deviatoric strain) while a positive $\tilde{\zeta}_1$, denoting contractile active stresses, destabilise systems in which the nematogens align perpendicular to the local deviatoric strain anisotropy. More interestingly, if the magnitude of $\tilde{\zeta}_2$ is larger than $2\tilde{\zeta}_1/S_0$, it always destabilises the orientationally ordered state. Therefore, here $\tilde{\zeta}_2$ plays a *destabilising* role in contrast to incompressible active fluids on substrates, where it may also play a *stabilising* role.

We now show that when the nematic elastomer is stable, the static structure factor of both $u_x$ and $u_y$ fluctuations scale as $1/q^2$ in *all* directions of the Fourier space. Introducing uncorrelated white noises of strength $2T$ in both the equations, we obtain

$$\langle u_x(q,t)u_x(-q,t)\rangle = \frac{T}{(\nu_1+\nu_4)q_x^2 + (\nu_2+\nu_5)q_y^2}\left[1 + \frac{\nu_3^2 q_x^2 q_y^2 + (\nu_4 q_x^2 + \nu_5 q_y^2)^2}{\nu_1\nu_4 q_x^4 + \nu_2\nu_5 q_y^4 + (\nu_2\nu_4 + \nu_1\nu_5 - \nu_3\nu_6)q_x^2 q_y^2}\right] \tag{67}$$

$$\langle u_y(q,t)u_y(-q,t)\rangle = \frac{T}{(\nu_1+\nu_4)q_x^2+(\nu_2+\nu_5)q_y^2}\left[1+\frac{\nu_6^2 q_x^2 q_y^2+(\nu_1 q_x^2+\nu_2 q_y^2)^2}{\nu_1\nu_4 q_x^4+\nu_2\nu_5 q_y^4+(\nu_2\nu_4+\nu_1\nu_5-\nu_3\nu_6)q_x^2 q_y^2}\right] \tag{68}$$

Both of these scale as $1/q^2$ in all directions of the wavevector space. It is easily checked however, that when the passive limit is taken with $\nu_2 = \nu_4 = 0, \nu_3 = \nu_6$, the correlation functions are highly anisotropic, with $\langle u_x u_x\rangle = T/[(\nu_1 - \nu_6^2/\nu_5)q_x^2]$ and $\langle u_y u_y\rangle = T/[(\nu_5 - \nu_6^2/\nu_1)q_y^2]$ scaling as $\mathcal{O}(1/q^4)$ along $q_y$ and $q_x$ respectively. Activity leads to a singular suppression of fluctuations with $\langle u_x u_x\rangle|_{q_x=0} = T/(\nu_2 q_y^2)$ and $\langle u_y u_y\rangle|_{q_y=0} = T/(\nu_4 q_x^2)$.

Note while we have focussed on two dimensional nematic elastomers, the calculation can be easily extended to three-dimensions by changing $q_y$ and $u_y$ to $q_\perp$ and $u_\perp$ where $\perp$ denotes the two directions transverse to the ordering direction $y, z$. There is also an additional elastic constant for $\eta_{xz}$ shears in the transverse plane in that case, but the rest of the calculation proceeds similarly.

## BIAXIAL NEMATIC ELASTOMERS

Biaxial nematic elastomers are softer than uniaxial nematic elastomers with vanishing elastic cost for $\eta_{xz}$ shears. Using the free energy (41) and a biaxial solution for $\mathbf{Q}_0$,

$$\mathbf{Q}_0 = \begin{pmatrix} -\frac{S_0}{3}+T_0 & 0 & 0 \\ 0 & -\frac{S_0}{3}-T_0 & 0 \\ 0 & 0 & \frac{2S_0}{3} \end{pmatrix} \tag{69}$$

we can calculate the fluctuations about the biaxial state:

$$\delta\mathbf{Q} = \begin{pmatrix} -\frac{\delta S}{3}+\delta T & 0 & 0 \\ 0 & -\frac{\delta S}{3}-\delta T & 0 \\ 0 & 0 & \frac{2\delta S}{3} \end{pmatrix} + \begin{pmatrix} 0 & 2T\theta_3 & (S-T)\theta_1 \\ 2T\theta_3 & 0 & (S+T)\theta_2 \\ (S-T)\theta_1 & (S+T)\theta_2 & 0 \end{pmatrix} \tag{70}$$

Just like in uniaxial elastomers, the Goldstone fluctuations $\theta_1$, $\theta_2$ and $\theta_3$ are slaved to strain fluctuations as $\theta_1 = [\mu/\{t(S_0-T_0)\}]\delta C_{xz}$, $\theta_2 = [\mu/\{t(S_0+T_0)\}]\delta C_{yz}$ and $\theta_3 = [\mu/(2tT_0)]\delta C_{xy}$. In passive biaxial elastomers integrating over $\theta_i$ also eliminates the harmonic energy cost for all shears. This implies that the passive force is of the form $f_i = -\alpha_1 q_i q_i u_i - \alpha_{ij} q_i q_j u_j$, where $i \neq j$. That is, there is no force proportional to $q_y^2 u_x$ or $q_z^2 u_x$ in $f_x$ and so on. Therefore, the static structure factor of $u_x$, $u_y$ and $u_z$ fluctuations all diverge logarithmically in two dimensions just as in smectics. However, as in uniaxial elastomers, activity restores these forces forbidden in equilibrium systems. Consider for simplicity a momentum-conserved biaxial elastomer. The active force is $\mathbf{f} = \nabla\cdot(\zeta_1\mathbf{Q} + \zeta_2\mathbf{Q}\cdot\mathbf{Q})$. This leads to active forces

$$f_x = i\left[\frac{2T_0}{3}(3\zeta_1 - 2S_0\zeta_2)q_y\theta_3 - \frac{1}{9}(3\zeta_1 - 2S_0\zeta_2 + 6T_0\zeta_2)q_x(\delta S - 3\delta T) + \frac{S_0-T_0}{3}(3\zeta_1 + S_0\zeta_2 + 3T_0\zeta_2)q_z\theta_1\right] \tag{71}$$

$$f_y = i\left[\frac{2T_0}{3}(3\zeta_1 - 2S_0\zeta_2)q_x\theta_3 - \frac{1}{9}(3\zeta_1 - 2S_0\zeta_2 - 6T_0\zeta_2)q_y(\delta S + 3\delta T) + \frac{S_0+T_0}{3}(3\zeta_1 + S_0\zeta_2 - 3T_0\zeta_2)q_z\theta_2\right] \tag{72}$$

$$f_z = i\left[\frac{S_0-T_0}{3}(3\zeta_1 + S_0\zeta_2 + 3T_0\zeta_2)q_x\theta_1 + \frac{2}{9}(3\zeta_1 + 4S_0\zeta_2)q_z\delta S + \frac{S_0-T_0}{3}(3\zeta_1 + S_0\zeta_2 - 3T_0\zeta_2)q_y\theta_2\right] \tag{73}$$

It is clear that replacing $\theta_i$ with the strains lead to forces $f_i \sim q_j q_j u_i$. Thus, as long as $(3\zeta_1 - 2S_0\zeta_2)$, $(3\zeta_1 + S_0\zeta_2 + 3T_0\zeta_2)$ and $(3\zeta_1 + S_0\zeta_2 - 3T_0\zeta_2)$ are all positive, activity leads to a singular stabilisation of the biaxial nematic elastomer – the static structure factor of $u_x$, $u_y$ and $u_z$ all remain finite in three dimensions, and they scale as $1/q^2$ in all directions of the wavevector space. One can follow through the programme developed for uniaxial systems and define a strain tensor and displacement fields for fluctuations about the biaxial state and obtain the equations of motion for these new displacement variables. However, that calculation is not very illuminating and we do not pursue it further here.

## REVIEW OF AND COMPARISON TO PASSIVE ELASTOMERS

In equilibrium, the dynamics of an orientationally ordered elastomer is controlled purely by a free-energy. The vanishing of a shear modulus in this case implies that one has to retain beyond harmonic terms in this free energy

the simplest of which is $(K/2)(\nabla^2\mathbf{u})^2$ (bending). It is known that phonon fluctuations destroy even quasi-long-range positional order in nematic elastomers in all dimensions below 3. A simple way of checking this is to write the free-energy of a nematic elastomer in Fourier space as $F = \frac{1}{2}\int \mathcal{G}_{ij}u_i(q)u_j(-q)$ with

$$\boldsymbol{\mathcal{G}} = \begin{pmatrix} B_1 q_x^2 + Kq^4 & (B_3/2)q_x q_y \\ (B_3/2)q_x q_y & B_2 q_y^2 + Kq^4 \end{pmatrix} \tag{74}$$

from which one can immediately calculate the equal-time correlators of the displacement field $\langle u_i(q,t)u_j(-q,t)\rangle = T\mathcal{G}_{ij}^{-1}$ where $T$ is the temperature. This yields the displacement correlations $\langle |u_x(q,t)|^2\rangle = T/[(B_1 - B_3^2/4B_2)q_x^2 + Kq^4]$ and $\langle |u_y(t)|^2\rangle = T/[(B_2 - B_3^2/4B_1)q_y^2 + Kq^4]$ Both of these diverge as a power of system size in two dimensions therefore destroying the ordered solid state. The angular fluctuations, which are slaved to displacement ones can however be seen to remain finite. In fact, in equilibrium two-dimensional systems the correlation of both $u_x$ and $u_y$ are exactly equivalent to two-dimensional smectics. This is of course not true in the presence of active stresses.

Extending the equilibrium model to three dimensions requires taking $u_y \to \mathbf{u}_\perp$, $q_y \to \mathbf{q}_\perp$, noting that there is a shear modulus for in-plane shears and therefore, writing the free energy $F = (1/2)\int \mathcal{G}_{ij}u_i(q)u_j(-q)$ with

$$\mathcal{G}_{\perp\perp} = (B_2 + B_4)q_{\perp i}q_{\perp j} + (B_4 q_\perp^2 + K_3 q_x^4)\delta_{ij} \tag{75}$$

$$\mathcal{G}_{x\perp} = (B_3/2)q_x q_\perp \tag{76}$$

$$\mathcal{G}_{xx} = B_1 q_x^2 + K_1 q_\perp^4 \tag{77}$$

One can them immediately check that the static structure factor of displacement fluctuations are

$$\langle u_x(q,t)u_x(-q,t)\rangle = \frac{T}{[B_1 - B_3^2/4(B_2 + 2B_4)]q_x^2 + K_1 q_\perp^4} \tag{78}$$

$$\langle \mathbf{u}_\perp(q,t)\mathbf{u}_\perp(-q,t)\rangle = \frac{T}{[(B_2 + 2B_4) - B_3^2/4B_1]q_\perp^2 + K_3 q_x^4}\mathsf{P}^L + \frac{T}{B_4 q_\perp^2 + K_3 q_x^4}\mathsf{P}^T \tag{79}$$

where the projection operators $\mathsf{P}^L = \hat{q}_\perp\hat{q}_\perp$ and $\mathsf{P}^T = \mathsf{I} - \hat{q}_\perp\hat{q}_\perp$ project parallel and transverse to the in-plane wavevector direction respectively. From this, one immediately notices that the $u_x$ fluctuations behave as in smectic liquid crystals diverging logarithmically even in three dimensions, while $\mathbf{u}_\perp$ fluctuations behave as in columnar systems and are finite in three dimensions. An equilibrium nematic elastomer is therefore like a combination of a smectic and a columnar phase. Note that this is simply due to the rotation invariance imposed vanishing of harmonic energy cost for $x$ $\perp$ shears. Furthermore, since $u_x$ fluctuations behave like smectic displacement fields, there are marginally relevant nonlinearities even in three dimensions. These nonlinearities arise from the requirement of rotation invariance – the linearised strain tensor is not rotation invariant. For this, the theory is written in terms of the correct rotation invariant strain tensor (after a suitable rescaling of $x$ and $u_x$) $\eta_{ij} = (1/2)(\partial_i u_j + \partial_j u_i - \partial_i u_x \partial_j u_x)$, $\eta_x = (\partial_x u_x + (1/2)\partial_i u_x \partial_j u_x$, where the indices $i$ and $j$ denote directions transverse to the ordering one. Rewriting the free energy as $\int B(\mathrm{Tr}[\boldsymbol{\eta}])^2 + C\mathrm{Tr}[\boldsymbol{\eta}]\tilde{\eta}_{pp} + (\mu_L/2)\tilde{\eta}_{pp}^2 + \mu\mathrm{Tr}[(\tilde{\boldsymbol{\eta}}_{\perp\perp})^2]$, where $\boldsymbol{\eta}$ is the full strain tensor, $\tilde{\boldsymbol{\eta}}$ is the deviatoric part of the strain tensor and $\eta_{pp}$ and $\boldsymbol{\eta}_{\perp\perp}$ are the projections along the ordering direction and purely transverse to it, one can show that all elastic coefficients other than $B$ (which goes to a non-universal value) vanish logarithmically at large scales and $\mu/\mu_L$ go to a universal value of 2. This implies that at large scales, equilibrium nematic elastomers are always incompressible [8]. Furthermore, $K_1$ diverges at large length scales (the divergences are algebraic below three dimensions). The large scale properties of three-dimensional equilibrium nematic elastomers are only different from the critical properties of three-dimensional smectics due to the presence of an in-plane shear modulus. If that were absent one could integrate out the $\mathbf{u}_\perp$ fluctuations to obtain a smectic free-energy in terms of $u_z$ (setting the irrelevant $K_3$ to 0). This is understandable since in that case the nematic elastomer is equivalent to a stack of liquid membranes. With the in-plane shear modulus, the nematic elastomer is equivalent to a stack of decoupled *solid* membranes and has the same critical behaviour.

However, all of this exotic physics is absent in active elastomers *even* in two dimensions. Activity, when stabilising, makes the static structure factor of both $u_x$ and $u_y$ fluctuations diverge as $1/q^2$ in *all* directions. Thus, it drastically suppresses the anisotropy of the fluctuation spectrum. Therefore, active elastomers have QLRO in two dimensions unlike their passive counterparts. Furthermore, in nematic elastomers, the simplest and lowest order nonlinearities

arise from the anharmonic terms in the rotation invariant strain tensor. They lead to terms of the form $\partial_x(\partial_y u_x)^2$ and $\partial_y(\partial_y u_x)^2$ in the equations of motion. The suppression of the anisotropic fluctuations also imply that these terms are irrelevant in two dimensions. The easiest way to see this is to note that at the linear fixed point, the anisotropy exponent is 1, while the roughness exponent for both $u_x$ and $u_y$ is $(2-d)/2 = 0$ in two dimensions and the dynamic exponent is 2. This immediately shows that all these nonlinearities are irrelevant. Therefore, the exotic physics that is obtained in passive nematic elastomers in three-dimensions is absent in active nematic elastomers even in two dimensions. This is equivalent to active smectic in two dimensions. Therefore, the linear theory presented here is the correct description of the QLRO phase of active nematic elastomers. We also note that though the three dimensional *equilibrium* nematic elastomer is equivalent to a stack of sliding solid membranes, the corresponding active problems are not equivalent. This is because symmetry forbids any term of the form $\partial_x^n \mathbf{u}_\perp$ both in the free energy and the equation of motion. Therefore, an active version of a lamellar phase of tethered membranes would not feature any force of the form $\partial_x^2 \mathbf{u}_\perp$.

Let us briefly discuss three-dimensional biaxial nematic elastomers now. In equilibrium, the free energy of a biaxial nematic elastomer is similar to the two-dimensional nematic elastomer in that the harmonic energy for both can be written as $\int \partial_i u_i \partial_j u_j$. This implies that, like two dimensional elastomers, biaxial elastomers can not resist shear in *any* direction. Therefore, the static structure factor for all three displacement variables are smectic-like in a biaxial elastomer.

In contrast to active nematic elastomers, two-dimensional polar elastomers have marginally relevant nonlinearities which we discuss now. Every nonlinearity of the form $(\nabla\mathbf{u})^2$ is marginally relevant in two dimensions. In fact, calculations for polar smectics suggest that the ordered phase is only realised when the coefficients of the only two nonlinearities allowed in that case $(\partial_z u)^2$ and $(\nabla_\perp u)^2$, where $u$ is the displacement of the smectic, have opposite signs. An equivalent calculation is however more difficult in our case due to the larger number of nonlinearities to keep track of. In general, one would expect nine nonlinearities with independent coefficients. However, the requirements of rotation invariance does restrict that to some extent. In the dynamics for $u_x$, the lowest order nonlinearities arise from three sources: i. from the rotation invariant strains $\eta_{xx}$ and $\eta_{yy}$, which would result in bilinear terms in the equations with coefficients related to the linear propulsive terms, ii. from the propulsive term $\mathbf{p}\cdot\mathsf{W}$ and iii. from additional propulsive terms of the form $\mathbf{p}\cdot(\mathsf{W}\cdot\mathsf{W})$. The nonlinearities in the $u_y$ equation arise from the term $\theta\partial_t u_x$. However, the considering the effects of these nonlinearities is beyond the scope of this paper and we leave it for future work. We note however, that polar smectics are possible in two dimensions (with a static structure factor that is qualitatively similar to the one obtained from the linear theory) when certain relations between the nonlinear coefficients hold and we hope that this is the case for active polar solids as well.

## ACTIVE ELASTOMER IN A MOMENTUM-CONSERVED FLUID

In this section we consider a (dilute) elastomer frictionally coupled with a permeating momentum conserved fluid. Writing the active forces as $\nabla\cdot\boldsymbol{\sigma}^a$, the elastic forces as $\nabla\cdot\boldsymbol{\sigma}^{el}$ and viscous forces of the fluid as $\nabla\cdot\boldsymbol{\sigma}^f$, we can write the coupled equations of the elastomer and the permeating fluid in the Stokes regime as

$$\nabla\cdot\boldsymbol{\sigma}^a + \nabla\cdot\boldsymbol{\sigma}^{el} + \Gamma_f(\Upsilon)(\mathbf{v}_p - \mathbf{v}_f) = 0 \tag{80}$$

$$\nabla\cdot\boldsymbol{\sigma}^f - \nabla\Pi - \Gamma_f(\Upsilon)(\mathbf{v}_p - \mathbf{v}_f) = 0 \tag{81}$$

where $\mathbf{v}_p$ is the elastomer velocity, $\mathbf{v}_f$ is the fluid velocity and $\Upsilon$ is the volume fraction of the elastomer. Incompressibility of the entire solution implies

$$\nabla\cdot(\rho_p\Upsilon\mathbf{v}_p + \rho_f(1-\Upsilon)\mathbf{v}_f) \approx \rho_f\nabla\cdot\mathbf{v}_f = 0 \tag{82}$$

where $\rho_p$ and $\rho_f$ are the densities of the elastomer and the fluid respectively. The final approximate equality is obtained using the approximation $\Upsilon \ll 1$ and $\rho = [\rho_p\Upsilon + \rho_f(1-\Upsilon)] \approx \rho_f$. Using the same approximation, we see that for dilute systems, the solvent velocity and the mass-averaged velocity $\mathbf{v}$ are approximately equal i.e., the incompressibility constraint can be taken to be $\nabla\cdot\mathbf{v} = 0$. From this, one can solve for $\mathbf{v}_p$

$$\mathbf{v}_p = \dot{\mathbf{u}} = \mathbf{v} + \Gamma_f^{-1}(\nabla\cdot\boldsymbol{\sigma}^a + \nabla\cdot\boldsymbol{\sigma}^{el}) = \mathbf{v} + \mathbf{v}_r \tag{83}$$

where $\mathbf{v}_r$ is the relative velocity of the elastomer with respect to the mean flow. Finally, the equation-of-motion for $\mathbf{v}$ is obtained by adding (80) and (81) (the drag forces cancel) yielding

$$\eta\nabla^2\mathbf{v} = \nabla\Pi - \nabla\cdot\boldsymbol{\sigma}^{el} + \nabla\cdot\boldsymbol{\sigma}^a = \nabla\Pi - \nabla\cdot\boldsymbol{\sigma} \tag{84}$$

where $\eta$ is the viscosity and $\nabla \cdot \boldsymbol{\sigma}$ is the sum of elastic and active forces. This is given by

$$\nabla \cdot \boldsymbol{\sigma} = [\tilde{\nu}_1 \partial_x^2 u_x + \tilde{\nu}_3 \partial_x \partial_y u_y + \tilde{\nu}_2 \partial_y^2 u_x]\hat{x} + [\tilde{\nu}_4 \partial_x^2 u_y + \tilde{\nu}_6 \partial_x \partial_y u_x + \tilde{\nu}_5 \partial_y^2 u_y]\hat{y} \tag{85}$$

where $\tilde{\nu}_i$ can be obtained from (60)-(65) by setting $\tilde{\zeta}_2 = 0$. We now project the displacement fields

$$u_t = \frac{q_y u_x - q_x u_y}{q} \tag{86}$$

transverse to and

$$u_l = \frac{\mathbf{q} \cdot \mathbf{u}}{q} \tag{87}$$

along the wavevector. Further, we use a stream function $\psi$ such that $v_x = \partial_y \psi$ and $v_y = -\partial_x \psi$, to rewrite the momentum equation taking the incompressibility constraint into account automatically. The transverse displacement field in terms of $\psi$ is

$$\dot{u}_t = \frac{iq^2\psi}{q} + \frac{q_y v_{rx} - q_x v_{ry}}{q} \tag{88}$$

while the longitudinal part of the displacement field is, of course, unaffected by the fluid

$$\dot{u}_l = \frac{\mathbf{q} \cdot \mathbf{v}_r}{q} \tag{89}$$

Solving for the velocity field, we obtain the following equation of motion for $u_t$:

$$\dot{u}_t = -\frac{1}{\eta}[\tilde{\nu}_4 \cos^4\phi + \tilde{\nu}_2 \sin^4\phi + (\tilde{\nu}_1 + \tilde{\nu}_5 - \tilde{\nu}_3 - \tilde{\nu}_6)] \cos^2\phi \sin^2\phi] u_t + \frac{\sin 2\phi}{2\eta}[(\tilde{\nu}_4 + \tilde{\nu}_6 - \tilde{\nu}_1)\cos^2\phi - (\tilde{\nu}_2 + \tilde{\nu}_3 - \tilde{\nu}_5)\sin^2\phi] u_l + \mathcal{O}(q^2) \tag{90}$$

Since $\dot{u}_l \sim \mathcal{O}(q^2)$, the eigenfrequency with $\mathcal{O}(q^0)$ leading part is

$$\omega = -\frac{1}{2\eta}\left[S_0\tilde{\zeta}_1(\beta^{-1} + \cos 2\phi) + (B_1 + B_2 - B_3)\frac{\sin^2 2\phi}{2} - \frac{\tilde{\zeta}_1 \sin^2 2\phi}{2\bar{w}}\{\Lambda_\parallel^2(t + sS0) - \Lambda_\perp^2(t - sS_0)\}\right] \tag{91}$$

where we have used the explicit expressions for $\tilde{\nu}_i$. This immediately implies that when $\beta^{-1} > 1$, $\tilde{\zeta}_1 \lesssim 0$ (extensile) the gel is unstable. This is clearly seen by setting $\phi = 0$ or $\phi = \pi/2$ in which case all but the first term of the eigenvalue vanishes, and the first term is destabilising. Similarly, for $\beta^{-1} < -1$, $\tilde{\zeta}_1 \gtrsim 0$ (contractile) the gel is unstable. The reason for this is that there is no passive restoring force fluctuations of $u_t$ either along or transverse to the wavevector direction due to the softness of the nematic elastomer.

Despite there being a relaxation rate proportional to $\mathcal{O}(q^0)$, the static structure factor of $u_t$ fluctuations scale as $1/q^2$ in all directions. To see this, one has to add thermal noise to (84) with the strength $2T\eta q^2$, which yields the static structure factor

$$\langle u_t(q,t) u_t(-q,t)\rangle = \frac{2T}{q^2}\left[S_0\tilde{\zeta}_1(\beta^{-1} + \cos 2\phi) + (B_1 + B_2 - B_3)\frac{\sin^2 2\phi}{2} - \frac{\tilde{\zeta}_1 \sin^2 2\phi}{2\bar{w}}\{\Lambda_\parallel^2(t + sS0) - \Lambda_\perp^2(t - sS_0)\}\right]^{-1}. \tag{92}$$

This implies that fluctuations in orientationally ordered gels are only logarithmically divergent in two dimensions.

These results were obtained after eliminating the angular fluctuations. Since orientational order is generically destabilised in active fluids, it may be natural to consider the coupled dynamics of orientational and positional fluctuations. Accordingly, we now assume that the fluctuations in the magnitude of the orientational order parameter are strongly suppressed and look at the coupled dynamics of orientational and positional fluctuations in a momentum conserved apolar elastomeric gel. Take the free energy

$$F = \frac{1}{2}\int d^2\mathbf{x} B_1 \eta_{xx}^2 + B_2 \eta_{yy}^2 + B_3 \eta_{xx}\eta_{yy} + B_4[\eta_{xy} - \beta(\theta - \Omega)]^2 \tag{93}$$

the velocity equation

$$-\eta\nabla^2\mathbf{v} = -\nabla\Pi + \tilde{\zeta}(\partial_y\theta\hat{x} + \partial_x\theta\hat{y}) - \frac{\delta F}{\delta\mathbf{u}} - \frac{1+\xi}{2}\partial_y\frac{\delta F}{\delta\theta}\hat{x} + \frac{1-\xi}{2}\partial_x\frac{\delta F}{\delta\theta}\hat{y} \tag{94}$$

where $\tilde{\zeta} = \tilde{\zeta}_1 S_0$ and the angle equation is

$$\dot{\theta} = \frac{1-\xi}{2}\partial_x v_y - \frac{1+\xi}{2}\partial_y v_x - \Gamma_\theta \frac{\delta F}{\delta \theta} = \frac{1-\xi\cos 2\phi}{2} q^2 \psi - \Gamma_\theta \frac{\delta F}{\delta \theta}. \tag{95}$$

Now solving for the velocity field in terms of the stream function $\psi$ we can write the effective dynamics of the angle field retaining the strains $\boldsymbol{\eta}$ and the rotation angle $\Omega$ for clarity:

$$\dot{\theta} = -2B_4\beta\Gamma_\theta[\beta(\theta-\Omega)-\eta_{xy}] - \frac{1}{8\eta}(\xi\cos 2\phi - 1)[2B_4\{\beta(\theta-\Omega)-\eta_{xy}\}(1+\beta\xi)\cos 2\phi - 2\tilde{\zeta}\theta + \{(2B_1-B_3)\eta_{xx} + (B_3-2B_2)\eta_{yy}\}\sin 2\phi] \tag{96}$$

This suggests that the assumption that the angle field quickly relaxes to a value given by the local strain may be incorrect for systems with large activity – at large activities, the system can be destabilised simply due to the generic instability, irrespective of the sign of the active coefficient. Note, that this obviously requires a description in terms of both the angle fields and the position variables since this instability could not have been detected in a description purely in terms of the position variables. To explore this instability more concretely, we again decompose the position fields in terms of the transverse $u_t$ and longitudinal $u_l$ fields. The coupled dynamics of $u_t$ and $\theta$ lead to two $\mathcal{O}(q^0)$ eigenvalues and we therefore only need to examine this. To lowest order, the equation for $u_t$ is

$$\dot{u}_t = \frac{i}{4q\eta}\left[2\cos 2\phi B_4(1+\beta\xi)\{\beta(\theta-\Omega)-\eta_{xy}\} - 4\tilde{\zeta}\cos 2\phi\theta + \{(2B_1-B_3)\eta_{xx} + (B_3-2B_2)\eta_{yy}\}\sin 2\phi\right] \tag{97}$$

The eigenvalues yielded by the coupled dynamics of $\theta$ and $u_t$ are generally complicated and we therefore calculate it only in a special case. We demonstrated that $\tilde{\zeta} > 0$ is stabilising for $\beta > 0$ in a description retaining only the displacement fields. Let us therefore take $\beta > 0$, $\tilde{\zeta} > 0$. Also, for simplicity, let us take $\xi = 0$. We know that active systems generating contractile stress (i.e. $\tilde{\zeta} > 0$) are maximally unstable along $\phi = \pi/2$ i.e. pure splay. Let us therefore calculate the $\mathcal{O}(q^0)$ part of the eigenvalue of the coupled $u_t$, $\theta$ dynamics in this case:

$$\omega = \frac{i}{8\eta}\left[2\tilde{\zeta} - B_4(1+4\beta^2\Gamma_\theta\eta) \pm \sqrt{\{2\tilde{\zeta} - B_4(1+4\beta^2\Gamma_\theta\eta\}^2 - 32B_4(1-\beta)\beta\Gamma_\theta\tilde{\zeta}\eta}\right] \tag{98}$$

We see that when $\tilde{\zeta}/\eta > B_4/2\eta + 2B4\beta^2\Gamma_\theta$, the system is destabilised. The quantity on the R.H.S. of this inequality is the effective relaxation rate of angular fluctuations in the absence of activity. This instability demonstrates that the orientational phase is destabilised at high values of the active forcing, irrespective of its sign, since the angle field is destabilised at a shorter timescale $\tau_a = (\tilde{\zeta}/\eta)^{-1}$ than is required for it to relax to the value given by the local strain. This presents an upper-limit on the value of the activity constant, irrespective of its sign, for which a description in terms of the displacement fields alone is sufficient.

Finally, we leave the steady Stokesian regime, restore inertia $\rho_0\partial_t\mathbf{v}$ and project the equations of motion along and transverse to the wavevector direction, ignoring viscosity as is appropriate in the long wavelength limit. We note that along $q_x = 0$ and $q_y = 0$, the equations of motion decouple and the sound speed for transverse ($u_t$) mode vanishes in passive elastomer as a consequence of vanishing restoring force for shear deformations. In contrast, in active systems that we have considered here, the sound speed of this mode along $q_x = 0$ is $\sqrt{S_0\tilde{\zeta}_1(\beta^{-1}-1)/2\rho_0}$ while along $q_y = 0$, it is $\sqrt{S_0\tilde{\zeta}_1(\beta^{-1}+1)/2\rho_0}$

## OTHER POSSIBLE STEADY STATES

In the main text we discussed the effects of activity on the equilibrium steady state that would have been obtained in a passive system. However, in nonequilibrium settings, infinitely many unique homogeneously ordered states are possible and there is no simple method to determine which state is chosen, since there is no free-energy whose minimisation leads to the most probable state. In particular, certain elastic moduli may vanish in some of these steady-states just as in equilibrium, even though the system contains active stresses. We now illustrate this in a model of apolar elastomer. We write the free-energy in (41):

$$F = \int d^2\mathbf{x}\left[\frac{\lambda}{2}\left(\Phi - \frac{s}{\lambda}Q_{ij}Q_{ij}\right)^2 + \mu\left(C_{ij} - \frac{t}{\mu}Q_{ij}\right)\left(C_{ij} - \frac{t}{\mu}Q_{ij}\right) + \frac{r}{2}Q_{ij}Q_{ij} + \frac{w}{4}(Q_{ij}Q_{ij})^2\right] \tag{99}$$

and the stress

$$\sigma_{ij} = \tilde{\zeta}_1 Q_{ij} + \frac{\delta F}{\delta \Phi}\delta_{ij} + \frac{\delta F}{\delta C_{ij}} \tag{100}$$

and we seek a homogeneously ordered steady state with $\delta F/\delta Q_{ij} = 0$, which is why we did not include terms depending on the molecular field conjugate to $Q_{ij}$ in the stress. Let us demand, in addition that $\sigma_{ij} = 0$. This is, of course, not required, but is not ruled out either. This results in

$$-2t\left(C^0_{ij} - \frac{t}{\mu}Q^0_{ij}\right) - s\left(\Phi^0 - \frac{s}{2\lambda}S_0^2\right)Q^0_{ij} + rQ^0_{ij} + \frac{wS_0^2}{2}Q^0_{ij} = 0, \tag{101}$$

$$\Phi^0 - \frac{s}{2\lambda}S_0^2 = 0, \tag{102}$$

and

$$2\mu\left(C_{ij} - \frac{t}{\mu}Q_{ij}\right) + \tilde{\zeta}_1 Q_{ij} = 0 \tag{103}$$

where

$$Q^0_{ij} = \frac{S_0}{2}\begin{pmatrix} 1 & 0 \\ 0 & -1 \end{pmatrix} \tag{104}$$

This implies that

$$C^0_{ij} = \frac{1}{\mu}\left(t - \frac{\tilde{\zeta}_1}{2}\right)Q^0_{ij} \tag{105}$$

which implies

$$\left(\frac{t\tilde{\zeta}_1}{\mu} + r + \frac{wS_0^2}{2}\right) = 0 \tag{106}$$

Now, we find that the angular fluctuations about this state are slaved to the strain fluctuations as

$$\partial_t\theta = \frac{4t\Gamma_Q}{2S_0}[-2C^0_{xx}\theta + \delta C_{xy}] \implies \theta = \frac{\mu}{(t - \tilde{\zeta}_1/2)S_0}\delta C_{xy} \tag{107}$$

The shear stress for fluctuations about this state is

$$\delta\sigma_{xy} = 2\mu\left(\delta C_{xy} - \frac{t}{\mu}\delta Q_{xy}\right) + \tilde{\zeta}_1\delta Q_{xy} = 2\mu\delta C_{xy} - 2\left(t - \tilde{\zeta}_1/2\right)S_0\theta = 0 \tag{108}$$

This implies that there is no restoring force for shears about this steady state. That is, though this system is active, the activity does not lead to a stiffening of fluctuations about this steady state. This demonstrates that it is possible to construct steady-states in which the modulus for shear in the plane containing the anisotropy axis is 0, just as in equilibrium, even in a system with active stresses. However, unlike in passive systems, this is not required by any symmetry and this state with vanishing shear modulus constitutes a measure 0 subspace in the space of all possible steady states. Therefore, a generic steady state of active orientationally ordered solids will have the dynamics we described in the main text. Further, in periodic active solids a possible selection criterion for the selection of steady state may be a vanishing dislocation speed in the steady state (an equivalent criterion is more difficult to formulate in the rubber-like solids we consider here). In a simpler model for active one-dimensional translation symmetry broken states (active smectics) we demonstrate that a vanishing dislocation speed will not, in general, have a vanishing tilt modulus which, as discussed earlier, is the analogue of the vanishing shear modulus of elastomeric solids. [5].

---

* nyomaitra07@gmail.com

[1] A. Maitra et al., in preparation
[2] T. C. Adhyapak, S. Ramaswamy, J. Toner, Phys. Rev. Lett. **110**, 118102 (2013)
[3] R. Lahiri, S. Ramaswamy, Phys. Rev. Lett. **79**, 1150 (1997)
[4] T. C. Lubensky et al., Phys. Rev. E **66**, 011702 (2002)
[5] A. Maitra et al., in preparation
[6] N Kumar et al. Nat commun. **5**, 4688 (2014)
[7] L. P. Dadhichi, A. Maitra, S. Ramaswamy, arXiv: 1808.08997
[8] X. Xing, L. Radzihovsky, Ann. Physics **323**, 105 (2008)
